# Supplementary material for: Geometric and General Relativistic Techniques for Non-relativistic Quantum Systems
Source: arXiv:2502.13009 source file (2025-02-18)
Supplement: Supplementary file 1 [file Appendix_Hom.tex]

\setcounter{secnumdepth}{-1}
\chapter{Appendix: Homology}
 %\chapter{Appendix: Homology}
%\section{Appendix: Homology}
\label{HomolAppendix}

Here we give a brief overview of the basic concepts, terminology and notation borrowed from the field of homology and used in the main body of this thesis. For a more complete description of homology theory and its relevance to lattice systems see \cite{Bombin_Chap,Browne_2014}. When we talk about the homology of a lattice in this thesis, we are specifically talking about a certain brand of homology known as $\mathbb{Z}_2$-homology. The central idea behind the homology of a lattice is to use the lattice to construct a family of vector spaces known as the homology groups. These homology groups contain information about the topology of the lattice they were constructed from.

In order to construct the homology groups from a lattice we first need to construct an auxiliary set of vector spaces known as the $p$-chain groups. A $p$-chain group is a vector space of $p$-dimensional objects which make up the defining lattice. We will only be considering two dimensional lattices here. Therefore, the only non-trivial $p$-chain groups we will discuss are the 0-chain, 1-chain and 2-chain groups related to the vertices, edges and faces of the lattice respectively. 

The $p$-chain groups are defined as follows: Given a lattice, we can consider the set of all vertices $V$, the set of all edges $E$, and the set of all faces (plaquettes) of the lattice $F$. The power set of $E$ can be given a vector space structure over the field $\mathbb{Z}_2$ by defining addition and scalar multiplication as follows. If $a,b\in P(E)$, we define the addition of $a$ and $b$ as follows (see Fig.~\ref{adding1chains}). 

\[ a+b = a \cup b \setminus a \cap b. \]
If $\lambda\in\mathbb{Z}_2$, we define scalar multiplication as:

\[ \lambda \cdot a = \left\lbrace
\begin{matrix}
a && \mbox{if $\lambda=1$} \\
\emptyset && \mbox{if $\lambda=0$}
\end{matrix} \right.
\]
It is straight forward to check that the tuple $(P(E),+,\cdot)$ forms a vector space with the empty set playing the role of the zero vector. As edges are one dimensional objects, an element of this vector space is known as a 1-chain and we denote the vector space by $C_1$. The power sets of $V$ and $F$ can also be given a vector space structure in the same way. Since vertices are zero dimensional objects, the vector space $(P(V),+,\cdot)$ is denoted by $C_0$, elements of which are called 0-chains. Similarly, as a lattice face is a two dimensional object, $C_2$ denotes the vector space $(P(F),+,\cdot)$ whose elements are called 2-chains.

\begin{figure}
\begin{center}
\includegraphics[scale=0.14]{Images/HomologyAppendix/figures/Adding1ChainsNew.png}
\end{center}
\caption{Depicted above is a graphical representation of the addition of two $1$-chains. As a 1-chain is a subset of $E$, we can represent it by colouring each edge which is an element of the 1-chain. Here, we have coloured an edge red if it is an element of the 1-chain and black if it not.}
\label{adding1chains}
\end{figure}

The next step in constructing the homology groups is to define the boundary operator $d_p$ for $p$-chains. The operator $d_p$ is defined to map a $p$-chain to the $(p-1)$-chain representing its boundary. For example, if $a$ is a 2-chain then $d_2a$ is the 1-chain that borders that 2-chain (See Fig.~\ref{BoundaryOp}). For $p$-chains with no boundary, the application of the boundary operator yields the zero vector in $C_{p-1}$. As of yet, there is no $C_{-1}$ group. However, it is clear that every 0-chain has no boundary and so the application of $d_0$, as defined, should yield the zero vector in $C_{-1}$. Hence, for $d_0$ to be well defined, it is usual to define $C_{-1}$ as a trivial vector space consisting of only a zero vector. It is an easy exercise to show the boundary operator is a linear operator. An obvious yet important property of the boundary operators is the following:

\[ d_{p-1} d_p = 0. \] 
where zero here is the operator which maps all $p$-chains to the zero vector in $C_{p-2}$. This simply states that a $(p-1)$-chain representing the boundary of a $p$-chain has no boundary. The subscript of the operator $d_p$ is often omitted in the literature as it is usually clear from context which boundary operator is being used.

\begin{figure}
\begin{center}
\includegraphics[scale=0.15]{Images/HomologyAppendix/figures/BoundaryOp.png}
\end{center}
\caption{Here, we show a graphical representation of the action the the boundary operator on 2-chains and 1-chains. We graphically represent 1-chains as we did in Fig.~\ref{adding1chains}. Similarly, as 2-chains are subsets of faces, we represent a 2-chain on a picture of the lattice by colouring its elements in blue. Likewise, we represent a 0-chain by colouring its elements in green. In the top two images we show an example of a 2-chain and its image under the boundary operator. In the bottom two images we show an example of a 1-chain and the 0-chain representing its boundary.}
\label{BoundaryOp}
\end{figure}

Within $C_1$ are two subspaces which will define the first homology group of the lattice. These are $Z_1\equiv \mbox{ker}(d_1)$ and $B_1\equiv \mbox{Im}(d_2)$. The first subspace, $Z_1$, is the vector space of 1-chains which have no boundary, known as 1-cycles. The second subspace, $B_1$, is the space of 1-chains which are the boundary of some 2-chain. We note that the subspace $B_1$ must also be a subspace of $Z_1$ since the following statements are equivalent:

\[ \mbox{Im}(d_2) \subset \mbox{ker}(d_1) \quad \mbox{ and } \quad
d_1 d_2 = 0.\]

We can define an equivalence relation $\sim$ on the space of 1-cycles using the space of boundaries by saying two 1-cycles are equivalent if their sum is the boundary of some 2-chain. That is, if $a,b \in Z_1$,

\begin{equation}
a \sim b \iff a+b \in B_1,
\end{equation}
in which case the cycles $a$ and $b$ are said to be homologous. The first homology group is then defined as the group of equivalence classes (or homology classes) under $\sim$, namely, the quotient space of $Z_1$ and $B_1$.

\begin{equation}
H_1 =  \faktor{Z_1}{B_1}.
\end{equation}
As both $Z_1$ and $B_1$ are vector spaces, $H_1$ is also a vector space. The equivalence class containing the zero 1-chain plays the role of the zero vector. Elements of this class represent the boundaries of 2-chains and are called homologically trivial. Non-zero elements of $H_1$ contain 1-cycles which are not the boundary of a 2-chain. Such 1-cycles can only exist if the underlying lattice has a one dimensional hole and in this way the first homology group $H_1$ of the lattice holds information about its topology.
